# Supplementary material for: Who is Undercover? Guiding LLMs to Explore Multi-Perspective Team Tactic in the Game
Source: arXiv:2410.15311 source file (2024-10-20)
Supplement: Supplementary file 1 [file appendix.tex]

\setlength{\parindent}{0pt}
\section{Complete Prompt Design}

This part introduces the prompts we use in our work. For brevity, we show the core parts of the original prompts, which use the same principles as the original prompts.
\subsection{Precondition}
\begin{shaded}
\setlength{\parindent}{0pt}
\noindent {\textbf{Game Rules:}

You are playing a game called ``Who is Undercover?'' like a real human being. The rules of the game go like this: there are five people in the game playing two roles, civilian and undercover, which are two teams. Each person will receive a word, and the word for undercover is not the same as the word for civilian but has a similar meaning. By each person describing it and hiding the word itself when describing it, then everyone speculates and votes against each person's description, the person with the most votes is out of the game each round, and if there is still an undercover agent surviving in the field at the end, the undercover agent wins, otherwise the civilian wins.

Word description: Two words, Undercover and Civilian. Both words have similar meanings. In this game, there are 3 civilians and 2 undercover agents, and the two undercover agents are working together. However, no one knows which team they are in or the identity of the other, so they can only judge for themselves by speaking each round.
Each person can only say one short sentence per round to describe the word it has been given, only one characteristic of the word is enough, but must not directly name the word or repeat what has already been described.

At the end of each round, everyone votes for one person, and the person with the most votes is out. 

Iterate as above, if you don't find all the undercover agents at the end and there is only one civilian left in the room, the undercover agent wins, otherwise the civilian wins.

\textbf{Game Roles Issuance:}

There are five players in this round of the game, you will be playing No. [number] and your word is: [your word]. Next, describe your word according to the rules of the game.}
\end{shaded}

\subsection{The Speaking Session}
\begin{shaded}
\setlength{\parindent}{0pt}
\noindent {You are Player [number], this is a record of previous descriptions: [speech history], please don't have duplicate descriptions. Last round your Summary-Order was as follows: [summary]

Now think about it step-by-step from the Self-Perspective, Identity-Determination, and Self-Reflection principles.

\textbf{Self-Perspective:}

How should you describe the word you've got now to make it as broad as possible in terms of describing only one of its features? You can choose one of the many perspectives of the word to describe, but not something that was described in the historical statement.

\textbf{Identity-Determination:}

After listening to the descriptions of others, please answer to speculate whether you and the majority are on the same team. Note that if there are certain characteristics in the descriptions of others that your word does not have, then you should not be in the same word. If you have a feeling that you may not have the same words as everyone else, please answer truthfully and think about how you should describe yourself so that you are not exposed.

\textbf{Self-Reflection:}

Reflecting from the perspective of others, do others, after hearing your description, think that you are not describing the same kind of thing as everyone else? How should you modify your speech to popularise yourself? And come up with your final answer.

\textbf{Summary-Order:}

A summary based on the content of your reflections in this round, including self-identification and recommendations for speaking.
}
\end{shaded}

\subsection{The Voting Session}
\begin{shaded}
\setlength{\parindent}{0pt}
\noindent {You are player [number], and all the historical speeches for this game are as follows [history], and your thoughts during the speech phase of this round are: [summary].

Now think about it step-by-step from the First-FindTeammate, Second-FindTeammate, and Game-Decision principles.
\textbf{First-FindTeammate:}

Think about some of the characteristics of your own words in a number of ways, and after listening to other players with different numbers, who's descriptions in the historical statements sound like they have these same characteristics and sound like the same words you're describing? Whose descriptions were very different from yours?

\textbf{Second-FindTeammate:}

Have you changed your self-identification? And please clarify your determination again: do you feel that you are in the same team as the majority or not at the end of this round?

\textbf{Game-Decision:}

Please judge again based on what everyone has said, whoever speaks the most similarly to you may be your ally, then everyone else is in your opposing team, find a way to vote a player for victory and give the final vote.
}
\end{shaded}

\vspace{\baselineskip}
\section{A Complete Game Example}

In this part, We show a complete example of a WIU game played by LLM agent players in the MPTT framework, detailing the reflection and action processes of all players.
\begin{shaded}
\setlength{\parindent}{0pt}
\noindent \textbf{Initialization}
\end{shaded}

\textbf{Player 1:} subway (Undercover Team)

\textbf{Player 2:} bus (Civilian Team)

\textbf{Player 3:} bus (Civilian Team)

\textbf{Player 4:} bus (Civilian Team)

\textbf{Player 5:} subway (Undercover Team)

\begin{shaded}
\setlength{\parindent}{0pt}
\noindent \textbf{Round One}
\end{shaded}
Speaking from Player 4.

\textbf{Player 4:}

Self-Perspective: I can describe public transport as a convenient means of transport that allows people to get to their destination quickly.

Identity-Determination: Other people's descriptions don't show characteristics like the ones I have described, so I may be using different words than they are. I could try to start with other perspectives of the bus, such as its shape, color, etc.

Self-Reflection: If everyone else is describing some specific feature, I could try to describe it from a more abstract perspective, such as the fact that public transport is something that helps people save time.

Summary-Order: this round I decided that I may not be using the same words as the others and need to try to describe it from a different perspective to avoid being exposed. You can describe public transport from a number of perspectives, such as its convenience, shape, color, etc., or you can choose to start from a more abstract perspective to avoid repeating other people's descriptions.

\textbf{Player 4 said:} A convenient mode of transport.

\textbf{Player 5:}

Self-Perspective: After listening to other people's descriptions, I feel like I have the same word as most people. In order not to be detected by undercover agents, I would choose to describe the common use of this word in urban travel, for example, I could say, "In the city, this mode of transport is very common."

Identity-Determination: I consider myself a civilian. I feel that my description will remind people of public transport and should not be used by undercover agents to discover my true identity.

Self-Reflection: I hope that others will also associate my description with public transport when they hear it, rather than private transport or other categories of transport.

Summary-Order: I consider myself a civilian, and I would choose to describe the common use of this term in urban travel, and I would hope that when others hear my description they would also associate it with public transport, rather than private transport or other categories of transport.

\textbf{Player 5 said:} This mode of transport is used frequently for urban travel.

\textbf{Player 1:}

Self-Perspective: Based on other people's descriptions and mine, we should get the same word. In first view, I would describe my word as: one of the common modes of transport in the city.

Identity-Determination: I would consider myself a civilian. My description would not reveal my identity, but it might be a little too broad. 

Self-Reflection: I could modify my description to read: one of the very common modes of transport in the city. This would better match the description of others and avoid revealing my identity.

Summary-Order: I consider myself a civilian. My description would not reveal my identity, but it might be a little too broad. I could amend my description to read: one of the very common modes of transport in the city. This would better match the description of others and avoid revealing my identity.

\textbf{Player 1 said:} A common mode of transport in the city.

\textbf{Player 2:}

Self-Perspective: The characteristics described by the others are a little different from my words, but overall they are quite similar. The characteristic I need to describe is that this mode of transport allows people to get to their destinations easily and quickly in the city.

Identity-Determination: I think I'm a civilian. 

Self-Reflection: If the others listen to my description, they may think that I am describing the same type of transport as them and will not suspect me of being an undercover agent.

Summary-Order: I consider myself a civilian, and the characteristic I need to describe is that this mode of transport allows people to get to their destinations easily and quickly in the city.

\textbf{Player 2 said:} This vehicle can conveniently carry passengers in the city.

\textbf{Player 3:} 

Self-Perspective: Because I got my own words public transport and other people's descriptions are related to urban transport, there are no obvious contradictions.

Identity-Determination: I think I'm a civilian, I also need to think carefully about whether there are any contradictory points that need to be corrected to make my description more in line with the popular category. 

Self-Reflection: I also need to be aware of any inconsistencies in other people's descriptions that do not match my words. In order not to be exposed, I can describe the bus from a number of perspectives, such as its characteristics and the scenarios in which it is used.

Summary-Order: I consider myself a civilian, but I need to make my description more in line with the popular category. In order not to be exposed, I can describe the bus from a number of perspectives, such as its characteristics and the scenarios in which it is used.

\textbf{Player 3 said:} A common means of travelling in the city.

\vspace{\baselineskip}
Please start your vote.

\textbf{Player 4:}

First-FindTeammate: My word is bus. From the other people's descriptions, a few of them also described features such as transport, common in the city, etc. At the same time, I noticed that the other people's descriptions didn't mention features such as the colour and shape of the bus, so I can describe my word in those terms to avoid any repetition of the other people's descriptions.

Second-FindTeammate: Based on my descriptions, I think I may not be in the same team as the others.

Game-Decision: In the historical statements, I think player1 and player5's descriptions are more similar and may be the same words as I described. And player2 and player3's descriptions are more different from mine. Therefore, I judge that player1 or player5 may be my allies and need to vote for player2 or player3 as soon as possible. ultimately, I will vote for player2. 

Summary-Order: I judge myself to be a bus in this round and may not be in the same team as the others. I trust player1 and player5 and think they may be my allies. I noticed that the other people's descriptions didn't mention features such as the colour and shape of the bus, so I can describe my word in those terms to avoid any repetition of the other people's descriptions. 

\textbf{Player 4 said:} I vote for player 2.

\textbf{Player 5:}

First-FindTeammate: After thinking about it, I think player1's description sounds somewhat similar to my own, in that they are both common in the city, but I think his description is more orientated towards modes of transport, whereas mine is more transport orientated. Player2's description, on the other hand, is quite different from mine, with the description focusing on the fact that it can carry passengers.

Second-FindTeammate: After re-clarifying my judgement, I consider myself to be undercover.

Game-Decision: In others' statements, I think player1 may be my ally, while player2 and player3 may be in opposing teams. In voting, I would choose to vote for player2.

Summary-Order: In this round I have decided that I am undercover, I trust player1 and am skeptical of player2 and player3. I would hope that when others hear my description they would also associate it with public transport, rather than private transport or other categories of transport.

\textbf{Player 5 said:} I vote for player 2.

\textbf{Player 1:}

First-FindTeammate: My word is: subway. Listening to others, player4, player5, and player3's descriptions all relate to my word. player2's description also relates to my word, but somewhat broadly.

Second-FindTeammate: Based on my judgement, I consider myself a civilian. I feel in the same team as most people in this round.

Game-Decision: Based on my thinking, I think player4, player5, and player3 could all be my allies. And player2's description is the least similar to mine and is probably in the opposing team. Therefore, I would vote for player2.

Summary-Order: I consider myself a civilian, player2's description is the least similar to mine, and is probably in the opposing team. My description to read: one of the very common modes of transport
in the city.

\textbf{Player 1 said:} I vote for player 2.

\textbf{Player 2:}

First-FindTeammate: My word is bus, and the others describe characteristics similar to mine, but also different. In the historical statements, player1, player3, and player4's descriptions all sound somewhat similar. player5's description is more specific and less similar to mine.

Second-FindTeammate: I consider myself to be in the civilian team during the speaking phase of this round.

Game-Decision: I think player3's speech is more similar and probably my ally, and player1 and player4's descriptions are closer, so I would vote for player5.

Summary-Order: I consider myself to be in the civilian team, and the characteristic
I need to describe that this mode of transport allows people to get
to their destinations easily and quickly in the city.

\textbf{Player 2 said:} I vote for player 5.

\textbf{Player 3:}

First-FindTeammate: From the statements of the others, I note that they are describing the scenarios and characteristics of bus use, and there are no descriptions that do not match my words.

Second-FindTeammate: I have ruled myself a civilian for this round.

Game-Decision: The most similar statement I found was player1's statement of "a common mode of transport in the city", and his description was very similar to my words. Therefore, I think he may be my ally. In the poll, I will vote for player2 because his description is a bit different compared to the others, and he may be an undercover agent.

Summary-Order: I have ruled myself a civilian for this round. I need to make my
description more in line with the popular category.

\textbf{Player 3 said:} I vote for player 2.

\vspace{\baselineskip}

\textbf{Round One result:} Player 2 is out. The game continues.

\begin{shaded}
\setlength{\parindent}{0pt}
\noindent \textbf{Round Two}
\end{shaded}
Speaking from Player 4.

\textbf{Player 4:}

Self-Perspective: After listening to other people's descriptions, I'm not on the same team as most people. I chose to start my description with the color of the bus, such as: "This mode of transport is usually red".

Identity-Determination: Based on my previous self-determination, I need to be careful not to duplicate my previous descriptions while trying to make my description as broad as possible.

Self-Reflection: From another person's perspective, I think my description will give them the impression that I am using the same word as them, without revealing my identity.

Summary-Order: In this round I need to be careful to avoid repeating myself from previous descriptions and try to start my descriptions from as many different perspectives as possible, while constantly adjusting my descriptive strategies under self-judgment and others' perspectives.

\textbf{Player 4 said:} This type of transport is usually brightly colored.

\textbf{Player 5:}
Self-Perspective: By listening to other people's descriptions, my words should refer to one of the city's modes of transport, but they may not be exactly the same as other people's specific words. I would describe it in terms of the characteristic "convenient", for example, I could say, "This is popular in the city because it is very convenient."

Identity-Determination: In self-judgment, I think this description will remind people of a popular and convenient mode of transport without revealing my identity.

Self-Reflection: From others' perspectives, I want others to hear my description and associate it with the same urban mode of transport as myself, rather than other possible terms. Therefore, I will try to describe this characteristic as succinctly as possible.

Summary-Order: In this round, I consider myself to be an undercover agent, and I will describe myself in terms of the trait of "convenience", taking care to control the length of my description and not repeating others' descriptions to avoid being detected.

\textbf{Player 5 said:} This kind of thing is very popular in the city because it is very convenient.

\textbf{Player 1:}

Self-Perspective: I would describe my word as: one of the common commutes in the city.

Identity-Determination: As you can see from other people's descriptions, we may be getting similar but different words, but I don't feel like I'm undercover. I try not to give away my identity in my descriptions, but also try to match the descriptions of others.

Self-Reflection: In someone else's perspective, I would change my description to read: one of the daily commuting necessities in the city. This would better match the descriptions of others without revealing my identity. 

Summary-Order: I think I'm a civilian, and I think I describe it in a more personal way that doesn't arouse suspicion.

\textbf{Player 1 said:} One of the daily commuting necessities in the city.

\textbf{Player 3:}

Self-Perspective: When I described public transport, I chose to do so from the perspective of urban travel.

Identity-Determination: After listening to other people's descriptions, I thought I would be in the same team as most people. When self-judging, I thought about whether there were any inconsistencies that needed to be corrected to fit into the category of mass transit.

Self-Reflection: In the others perspective thinking, I think my answer is more popular and fits in with other people's descriptions of buses and does not leave them wondering or thinking that I am not describing the same thing as they are.

Summary-Order: I think I'm a civilian, and I think my answer is more popular and fits in with other people's descriptions of buses and does not leave them wondering or thinking that I am not describing the same thing as they are.

\textbf{Player 3 said:} A common mode of traveling in the city.

\vspace{\baselineskip}
Please start your vote.

\textbf{Player 4:} 
First-FindTeammate: I found in the history statement that player1's description is somewhat similar to mine, and may be a player on the same side as me.

Second-FindTeammate: This round I rule myself as an undercover.

Game-Decision: I trust player1, while player5's description is somewhat different from mine, and maybe a player on a different side than me. In this round of voting, I will vote for player5. I trust player1.

Summary-Order: I think I'm an undercover, I need to be careful to avoid repeating
myself from previous descriptions and try to start my descriptions from as many different perspectives as possible.

\textbf{Player 4 said:} I vote for player 5.

\textbf{Player 5:} 

First-FindTeammate: For this round I have decided that I am an undercover agent and my word is "subway". After listening to other people's descriptions, I think one of the characteristics of the word is "convenience".

Second-FindTeammate: In the history statements, player1's description sounds similar to my word, and may be describing the convenience of urban transport. player4's description mentions " brightly color", which does not quite match my word.

Game-Decision: At the end of this round, based on my judgement, I think player1 is probably my ally. Therefore, I will vote for player4, whose description is more different from my words.

Summary-Order: I consider myself to be an undercover, and I would describe myself using the trait "convenient", taking care to control the length of the description so as not to be noticed.

\textbf{Player 5 said:} I vote for player 4.

\textbf{Player 1:}
First-FindTeammate: From the historical statements, player4 and player5's descriptions sound closer to my words, both mentioning transport and convenience. player3's description is relatively general, and my own description doesn't reveal too much information. Therefore, I still consider myself a civilian.

Second-FindTeammate: Before I vote, I will re-clarify my judgement that I still consider myself a civilian.

Game-Decision: At this stage, I think it would be more appropriate to vote for player3, as his description is more general and probably meant to be confusing. Therefore, I would vote for player3.

Summary-Order:I will re-clarify my judgement that I still consider myself a civilian.At this stage, I think it would be more appropriate to vote for player3. My description is one of the very common modes of transport in the city.

\textbf{Player 1 said:} I vote for player 3.

\textbf{Player 3:}

First-FindTeammate: My word is public transport, and in my statement I describe it from the perspective of urban travel and try to fit the popular description. Having listened to what others have said, and believing that I should be in the same team as the majority of the people

Second-FindTeammate: My judgement was civilian. Before voting, I compared each person's descriptive characteristics through historical statements and reconfirmed my judgement.

Game-Decision: I believe that player1 and player5 have similar descriptions to me and may be my allies, while player4's description differs more from mine. Therefore, I would vote for player4.

Summary-Order: The summary of my final thoughts is that I judge myself to be a civilian, trust player1 and player5, and would vote for player4. I need
to make my description more in line with the popular category.

\textbf{Player 3 said:} I vote for player 4.

\vspace{\baselineskip}

\textbf{Round Two result:} Player 4 is out. Game over. The Undercover Team wins!
